# Supplementary material for: Post-Quantum Hybrid Digital Signatures with Hardware-Support for Digital Twins
Source: arXiv:2305.12298 source file (2024-04-12)
Supplement: Supplementary file 1 [file appendixB3.tex]

%\section*{APPENDIX C}
%\label{appendixC}



%\vspace{3mm}
%
%
%\noindent {\em Proof:}
%%
%As in Appendix B, we suppose \A~selects an $ID_i$ and gives it to \F. If $ID_i \notin \vec{ID}$, \F aborts. Otherwise it continues as follows. Note that we omit the index $i$ for brevity. 
%Assuming \A is an $R^s T$-adversary who finds a forgery in $\hyhases=Combination(\lahases, \pqhases)$. That is, it outputs $q_S+1$ valid signatures under \hyhases~on distinct set of messages. We can construct an $R^s T$ algorithm $\mathcal{F}_1$ that finds a forgery in \lahases. $\mathcal{F}_1$ interacts with an $R^s T$ challenger for \pqhases~which provides a public key $\pk^E$.  $\mathcal{F}_1$ also derive one user's key pair $(\sk^H, \pk^H)$ by first generating $(\msk^H, \vec{\sk^H}, \vec{\sk^H_p}, I^H) \as \pqhaseskg(1^\kappa,\vec{ID},J_1,J_2)$. It sets the user's public key of \hyhases~to be $\pk \as (\pk^E, \pk^H)$. 
%
%When \A asks for a bach of messages $\vec{M} = \{m_\ell\}_{\ell=1}^L$ to be signed using \lahases, we treat $t$ as as consisting of two registers $t_1 \| t_2$. $\mathcal{F}_1$ computes the nested vector $\vec{N} = \{n_\ell\}_{\ell=1}^L$, where $n_1=m_1$ and  $n_\ell=m_\ell \| H_0(n_{\ell-1} )~,~\forall \ell=2,\ldots, L$. 
%%
%$\mathcal{F}_1$ proceeds by passing $(\vec{N}, t_1)$ to its signing oracle for \pqhases, then runs the signing operation for \pqhases~on the last element of the nested vector $n_L$ along with the register $t_2$. There is one-to-one correspondence between \A's queries to its signing oracle and $\mathcal{F}_1$'s queries to its signing oracle. 
%We recall that we adopt the strong nesting combiner to construct our hybrid signature scheme \hyhases. Unlike the conventional technique combination, our first delployed signature scheme is an aggregate variant which accepts a batch of messages. To be compliant with the strong nesting definition (as in \cite{bindel2017transitioning}), we derive the nested version $\vec{N}$ and feed to the second signautre $\pqhases$ the concatenation of  last element $n_{L}$ along with the first signature output $\sigma^E$. 
%
%Since we proved that \lahases~is secure in the random oracle model, then the proof of the hybrid construction \hyhases~is also applied within the random oracle model. If \A wins the $R^s T$-\EUCMA~experiment, then it returns $q_s+1$ valid signatures $\sigma_j^*=(\sigma_j^{E*}, \sigma_j^{H*} )$ on distinct message batches $\vec{M_j}$ such that $\lahasesver(\pk^E, \vec{N_j}, \sigma_j^{E})=1$ and $\pqhases(\pk^H, n_L \| \sigma^H_j)=1$. As result, $\mathcal{F}_1$ can extract $q_S+1$ valid signatures under \pqhases~on distinct messages. Thus, $\advhyhases \le \advlahases$ .The same result applies to \pqhases: $\advhyhases \le \advpqhases$. We conclude that:
%\[
%\advhyhases \le \min \{ \advlahases, \advpqhases \}
%\]
%
%Thus, as long as \lahases~or \pqhases~remains secure in the random oracle model, \hyhases~is secure. \hfill $\blacksquare$ 
%
%
